# Supplementary material for: Coloring problems on arrangements of pseudolines
Source: arXiv:2402.12564 source file (2024-02-19)

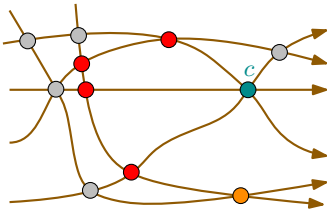

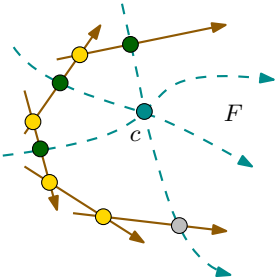

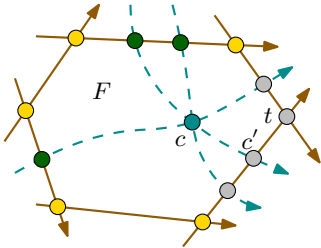

Supplement: Supplementary file 1 [file conflict_ancestors_appendix.pdf]
